# Supplementary material for: Predictive Sampling with Forecasting Autoregressive Models
Source: arXiv:2002.09928 source file (2020-07-08)
Supplement: Supplementary file 1 [file forecasting_capacity.tex]

\section{Capacity of forecasting modules}

We perform a small ablation study where we increase the number of channels for the forecasting modules.
In each case, a forecasting module consists of a strictly triangular 3x3 masked convolution followed by a 1x1 convolution.
We sample 10 batches using batch size 1. 

% Num channels  &                                    
%           18  & 40.8\std{4.1} & 61.5\std{6.2}                                   
%               & 20.7\std{2.7} & 30.4\std{3.9}
%           36  & 37.9\std{7.2} & 56.4\std{10.6}     
%               & 21.1\std{1.8} & 30.7\std{2.5}      
%           81  &               & 
%               &               & 
%           162 &               & 
%               &               & 
%           324 & 39.1\std{6.4} & 58.3\std{9.2}
%               & 20.8\std{2.6} & 30.1\std{4.0}
% 
%  
